# Supplementary material for: Unlocking Pixels for Reinforcement Learning via Implicit Attention
Source: arXiv:2102.04353 source file (2021-10-02)
Supplement: Supplementary file 1 [file appendix_2.tex]

\section{Theoretical Results}

\subsection{Function $P$}
As wee mentioned above, function $P$ can for instance produce a permutation matrix that sorts the entries of the input of $P$ from largest to smallest. Function $P$ can be also learnable. Regardless of whether it is learnable or not, it is useful to think about it as a result of the flow conducted on the orthogonal group $\mathcal{O}(\mathbb{R}^{(a \cdot b) times })$ (note that the permutation group $\mathrm{Perm}(\mathbb{R}^{(a \cdot b) \times (a \cdot b)})$ is a subgroup of $\mathcal{O}(\mathbb{R}^{(a \cdot b) times })$). 
We rewrite $P(\mathbf{r}^{\top}\mathbf{A}_{K})$ as the value of the flow on $\mathcal{O}(\mathbb{R}^{(a \cdot b) \times (a \cdot b)})$ defined as:
\begin{equation}
\label{eq:flow}
\frac{d\mathbf{P}(t)}{dt} =  \mathbf{P}(t)[\mathbf{P}(t)^{\top}\mathbf{Q}\mathbf{P}(t),\mathbf{N}],   
\end{equation}
where $\mathbf{Q},\mathbf{N} \in \mathbb{R}^{(a \cdot b) \times (a \cdot b)}$ are parameter matrices
and $[]$ stands for the \textit{Lie bracket} defined as follow: $[\mathbf{U},\mathbf{W}] = \mathbf{UW} - \mathbf{WU}$. For instance, if $\mathbf{Q}=\mathrm{diag}([1,...,(a \cdot b)])$ and $\mathbf{N} = \mathrm{diag}(\mathbf{r}^{\top}\mathbf{A}_{K})$ then $\mathbf{P}(t)$ converges to a permutation matrix that sorts the entries of the input of $P$ from largest to smallest. 
To integrate the flow given in Equation \ref{eq:flow}, we discretize this equation and update its discretized version as follows:
\begin{equation}
\label{eq:discr}
\mathbf{P}_{i+1} = \mathbf{P}_{i}\exp(\eta \Omega_{i}),    
\end{equation}
where $\eta > 0$ is a step size and $\Omega_{i}$ is a skew symmetric matrix defined as:
\begin{equation}
\Omega_{i} = [\mathbf{P}_{i}^{\top}\mathbf{Q}\mathbf{P}_{i},\mathbf{N}] \in \mathbb{R}^{(a \cdot b) \times (a \cdot b)}.    
\end{equation}
Computation of $\exp(\eta \Omega)$ is in practice intractable, thus we replace it with $\exp(\eta \widehat{\Omega})$, where: $\widehat{\Omega}=(a \cdot b)^{2} \Omega_{k_{r},l_{r}} \mathbf{H}_{k_{r},l_{r}}$, $k_{r},l_{r}$ is a random pair of two different indices (without loss of generality we assume that $k_{r} < l_{r}$) and $\mathbf{H}_{k,l}$  is a matrix such that $\mathbf{H}_{k, l} = 1$, $\mathbf{H}_{l,k}=-1$ and $\mathbf{H}$ is equal to $0$ otherwise. Note that $\widehat{\Omega}$ is an unbiased estimation of $\Omega$. It turns out that $\exp(\eta \widehat{\Omega})$ can be rewritten as $\mathbf{G}_{k_{r},l_{r}}(\eta  (a \cdot b)^{2}\Omega_{k_{r},l_{r}})$, where $\mathbf{G}_{k,l}(\theta)$ stands for the Givens rotations in the $2$-dimensional subspace given by canonical vectors $\mathbf{e}_{k},\mathbf{e}_{l}$ and of angle $\theta$. Thus we replace the update given in Equation \ref{eq:discr}, by the following one:
\begin{equation}
\mathbf{P}_{i+1} = \mathbf{P}_{i}\mathbf{G}_{k^{i}_{r},l^{i}_{r}}(\theta),    
\end{equation}
where: $(k^{i}_{r},l^{i}_{r})$ is a random pair of different sorted indices in iteration $i$ and $\theta=\eta  (a \cdot b)^{2}\Omega_{k^{i}_{r},l^{i}_{r}}$. It turns out that $\mathbf{P}_{i}$s obtained in this way can be inserted to the attention module defined by Equation \ref{eq:attention} in a way that still supports efficient computation of the entire block.
